# Supplementary material for: Minimal Lattice Model of Lipid Membranes with Liquid-Ordered Domains
Source: arXiv:2103.13761 ancillary file (2021-10-25)
Supplement: Supplementary file 1 [file si.pdf]

# Supplemental Material for
# "Minimal Lattice Model of Lipid Membranes with Liquid-Ordered Domains"

Tanmoy Sarkar[1] and Oded Farago[1,*]

[1]*Department of Biomedical Engineering, Ben Gurion University of the Negev, Be'er Sheva 84105, Israel*

(Dated: August 1, 2021)

## I. LATTICE SITE CLASSIFICATION ALGORITHM

We employ the following algorithm to categorize the lattice sites into gel, $L_o$ and $L_d$. Recall that each site can be in one of four states: void ($s = 0$), disordered DPPC chain ($s = 1$), ordered DPPC chain ($s = 2$), and Chol ($s = 3$).

Step 1: Sites in $s = 2$ state with six neighbors also in $s = 2$ state are labeled as gel.

Step 2: Sites in $s = 2$ state with three to five neighbors in $s = 2$ state are labeled as $L_o$.

Step 3: Unlabeled sites in $s = 2$ or $s = 3$ states that are neighbors of sites labeled gel or $L_o$, are labeled $L_o$.

Step 4: Unlabeled site in $s = 2$ state with two neighbors in $s = 2$ state and two and more neighbors in $s = 3$ state are labeled $L_o$.

Step 5: Unlabeled sites in $s = 2$ or $s = 3$ states that are neighbors of sites labeled $L_o$, are labeled $L_o$.

Step 6: Unlabeled sites in $s = 2$ state are labeled $L_d$.

Step 7: Unlabeled sites in $s = 3$ state that are neighbors of sites labeled $L_o$, are label $L_o$.

Step 8: Unlabeled sites in $s = 3$ state are labeled $L_d$.

Step 9: Sites in $s = 1$ state with three or more neighbors in $s = 0$ and $s = 1$ states are labeled $L_d$.

Step 10: Unlabeled sites in $s = 0$ or $s = 1$ states that are neighbors of sites labeled $L_d$, are labeled $L_d$.

Step 11: Unlabeled sites in $s = 0$ state with three or more neighbors in $s = 0$ and $s = 1$ states are labeled $L_d$.

Step 12: Unlabeled sites in $s = 0$ or $s = 1$ states that are neighbors of sites labeled $L_d$, are labeled $L_d$.

Step 13: Unlabeled sites in $s = 0$ or $s = 1$ states are labeled $L_o$.

The order of some of the steps may be interchanged (e.g., steps 6 and 7, steps 10 and 11, steps 9 and 11), but we have verified that this would cause only a few sites on the lattice to be labeled differently.

## II. STABLE, WEAKLY STABLE, AND UNSTABLE ORDERED CHAINS IN $L_o$ REGION

We consider the system just slightly above the main melting transition temperature $k_BT_m = 0.9\epsilon$. As above, the different states of the sites are denoted by $s = 0, 1, 2, 3$ for voids, disordered lipid chain, ordered lipid chains, and Chol, respectively. For the model parameters $\Omega_1 = 3.9$, $\epsilon_{22} = 1.3\epsilon$, and $\epsilon_{23} = 0.72\epsilon$, an exchange of the state of a lipid chain from ordered ($s = 2$) to disordered ($s = 1$) would:

1. Increase the system's energy by $\Delta E > k_BT$ if the chain has (i) four or more neighbors in state $s = 2$, (ii) three neighbors in state $s = 2$ and at least one neighbor in state $s = 3$, (iii) two neighbors in state $s = 2$ and at least three neighbors in state $s = 3$, or (iv) one neighbor in state $s = 2$ and five neighbors in state $s = 3$. We define an ordered chain satisfying one of these criteria as "stable".

* ofarago@bgu.ac.il

2. Increase the system's energy by $0 < \Delta E < k_BT$ if the chain has (i) three neighbors in state $s = 2$, (ii) two neighbors in state $s = 2$ and two neighbor in state $s = 3$, or (iii) one neighbor in state $s = 2$ and four neighbors in state $s = 3$. We define an ordered chain satisfying one of these criteria as "weakly stable".

3. Decrease the system's energy by $\Delta E < 0$ in all other cases. Such an ordered chain is "unstable".

Fig. S1(a) shows a snapshot from the simulations featuring $L_o$ domains with gel-like clusters and surrounded by a $L_d$ membrane. For most of the sites, we use the same color coding as in fig. 1 in the main text, i.e., white, blue, green, and red for states $s = 0, 1, 2, 3$, respectively. The only exception are the ordered DPPC chains ($s = 2$) in the $L_o$ regions, which are marked with yellow borders [as in fig. 1(h1,h2) in the main text] and, instead of green, are colored with black, magenta, and deep blue for stable, weakly stable, and unstable chains, respectively. In the snapshot, the majority of those chains are stable. Only a few weakly stable and unstable sites can be detected, mostly at the periphery of the domains. This explains the relative stability of the $L_o$ region, despite the fact that the gel and $L_d$ phases have a lower free energy. Fig. S1(b) shows the relative fractions of stable, weakly stable, and unstable chains as a function of Chol mole fraction $\chi$ at $T \simeq 1.01T_m$. The trends observed here indicate that the stability of the $L_o$ increases with $\chi$. Interestingly, the fraction of stable ordered chains saturates at a high level of about 0.9 when $\chi$ grows beyond the $L_d + L_o$ coexistence region in phase space [marked as the gray-shaded area in fig S1(b)]. This is consistent with the observation that at high Chol mole fractions, a single stable $L_o$ phase is formed.

## III. DYNAMICS

The SI movie (Movie_S1.mp4) is taken from the simulations of point "e" in the phase diagram (see fig. 1 in the main text) which is in the $L_d + L_o$ coexistence regime. The duration of the movie is about 100 $\mu s$ (see main text for the conversion of MC time units to physical ones). The characteristic life-times of the domains in the movie is $\lesssim 20\mu s$, indicating that thermodynamically the domains are meta-stable. This observation is consistent with the data from fig. S1(b) showing that at point "e" ($\chi \sim 0.17$), only 0.17 of the ordered chains in the $L_o$ region are unstable. As noted in the main text, dissociation of the domains is diffusion-limited. The main reason for the growth in the life times of the domains with $\chi$ is not the increasing stability of the ordered chains per se, but the concurrent growth in the size of the domains.

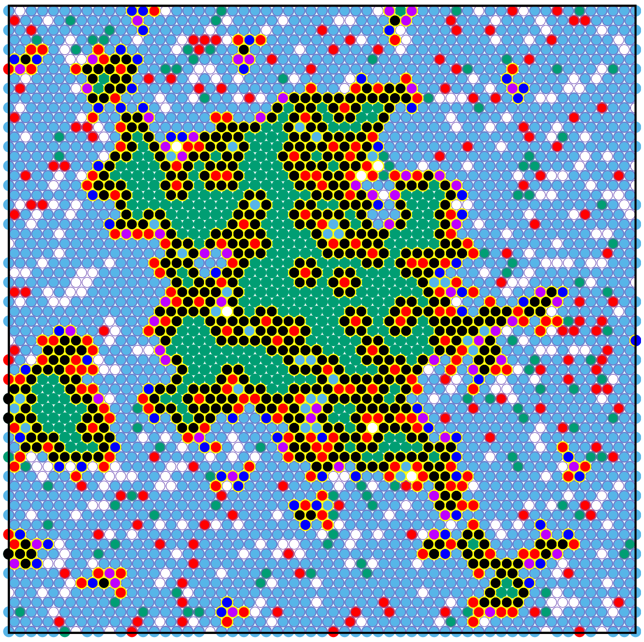

(a)

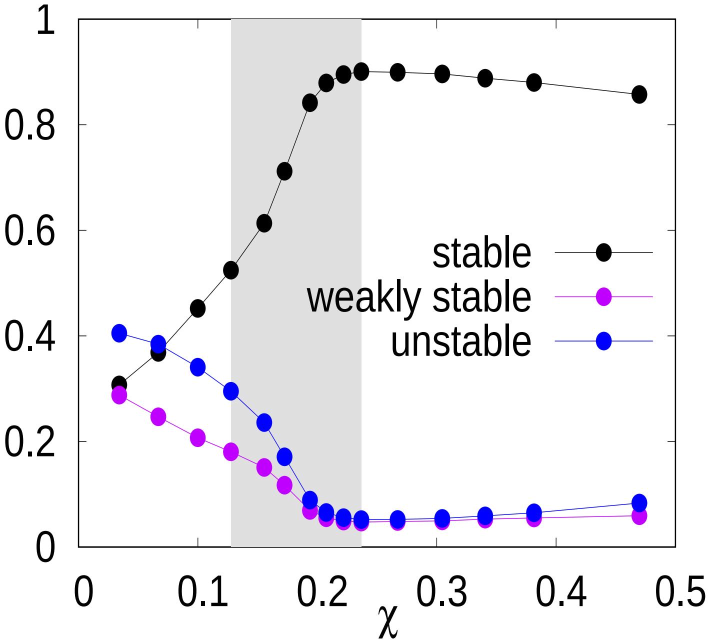


(b)

FIG. S1. (a) A snapshot from point "e" of the phase diagram, fig. 1 in the main text. The sites are colored according to their state and the region to which they belong. The regions are indicated by the color of the sites borders with purple, yellow, and no-color corresponding to $L_d$, $L_o$, and gel regions, respectively. The states are indicated by the colors of the sites interiors. Color coding for *most* sites is: white, blue, green, red for voids, disordered chains, ordered chains, and Chol, respectively. A different coding is used for the ordered chains in the $L_o$ region: black, magenta, and deep blue for stable, weakly stable, and unstable chains, respectively. (b) Relative fractions of stable, weakly stable, and unstable ordered chains in the $L_o$ region as a function of the Chol mole fraction at $T \simeq 1.01T_m$. The gray-shaded area marks the $L_d + L_o$ coexistence regime.
